# Supplementary material for: The extended Ville's inequality for nonintegrable nonnegative supermartingales
Source: arXiv:2304.01163 source file (2024-10-08)
Supplement: Supplementary file 1 [file supp.tex]

% Bornoullie -> Statistica Sinica

\documentclass[11pt]{article} % use larger type; default would be 10pt

\usepackage[utf8]{inputenc} % set input encoding (not needed with XeLaTeX)

\usepackage{cancel}

%%% Examples of Article customizations
% These packages are optional, depending whether you want the features they provide.
% See the LaTeX Companion or other references for full information.

%%% PAGE DIMENSIONS
\usepackage{geometry} % to change the page dimensions
\geometry{a4paper} % or letterpaper (US) or a5paper or....
\geometry{margin = 1.07 in} % for example, change the margins to 2 inches all round
% \geometry{landscape} % set up the page for landscape
%   read geometry.pdf for detailed page layout information

\usepackage{graphicx} % support the \includegraphics command and options
\usepackage[english]{babel}
% \usepackage[parfill]{parskip} % Activate to begin paragraphs with an empty line rather than an indent

%%% PACKAGES
\usepackage{booktabs} % for much better looking tables
\usepackage{array} % for better arrays (eg matrices) in maths
\usepackage{paralist} % very flexible & customisable lists (eg. enumerate/itemize, etc.)
\usepackage{verbatim} % adds environment for commenting out blocks of text & for better verbatim
\usepackage{subfig} % make it possible to include more than one captioned figure/table in a single float
\usepackage{amsfonts}
\usepackage{amssymb}
\usepackage{amsmath}
\usepackage{amsthm}
\usepackage{makecell}

\usepackage{epigraph}
\usepackage{bbm}

\usepackage{hyperref}
\hypersetup{
    colorlinks=true,
    citecolor=blue
}

\input{macros}

\usepackage[round]{natbib}
\bibliographystyle{abbrvnat}

\usepackage{wrapfig}
\usepackage{subfig}
\usepackage[capitalize,noabbrev]{cleveref}
\usepackage{authblk}
\usepackage{changepage}

\usepackage[21-]{pagesel}

%\title{Catoni-style confidence sequences\\for heavy-tailed mean estimation}
%\author[1]{Hongjian Wang}
%\author[2]{Aaditya Ramdas}
%\affil[1, 2]{Machine Learning Department, Carnegie Mellon University} 
%\affil[2]{Department of Statistics and Data Science, Carnegie Mellon University}
%\affil[ ]{\texttt{ \{hjnwang,aramdas\}@cmu.edu  }}

% \title{Nonintegrable Supermartingales\\ 
% and an Extended Ville's Inequality}
\title{Supplementary material to
\\ \large ``The extended Ville's inequality for nonintegrable nonnegative supermartingales''}
\author[*]{Hongjian Wang}
\author[*]{Aaditya Ramdas}
\affil[*]{Department of Statistics and Data Science, Carnegie Mellon University}
\affil[ ]{\texttt{ \{hjnwang,aramdas\}@cmu.edu  }}

%\date{\today} 
\date{\today}

\usepackage{tocbasic}
\DeclareTOCStyleEntry[
  beforeskip=.05em plus .6pt,% default is 1em plus 1pt
  pagenumberformat=\textbf
]{tocline}{section}

\begin{document}

\input{ENSM/main-sections.tex}
\input{ENSM/key-proofs.tex}
\input{ENSM/summary.tex}
\input{ENSM/ack.tex}
\newpage

\maketitle

\appendix
\input{ENSM/technical-bg.tex}
\input{ENSM/more-nsm.tex}
\input{ENSM/bayesian-ztest.tex}
\input{ENSM/more-proofs.tex}

\bibliography{ninsm}

\end{document}
